# Supplementary material for: Flatland Competition 2020: MAPF and MARL for Efficient Train Coordination on a Grid World
Source: arXiv:2103.16511 source file (2021-03-30)
Supplement: Supplementary file 1 [file architecture.tex]

\section{JBR\_HSE Solution Architecture}
\label{app:architecture}

\begin{figure}[!h]
    \centering
    \includegraphics[width=0.65\linewidth]{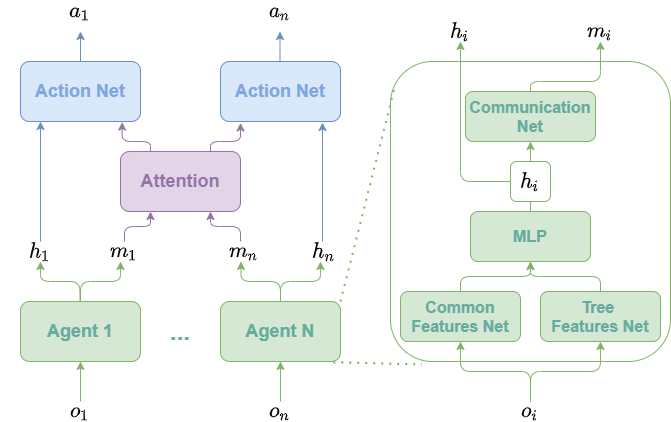}
    \caption{\textbf{Agent architecture.} $o, a, m$, and $h$ respectively denote observations, actions, messages, and extracted features.}
    \label{fig:architecture}
\end{figure}
